# Supplementary material for: Transferability of Atom-Based Neural Networks
Source: arXiv:2409.17575 ancillary file (2024-09-26)
Supplement: Supplementary file 1 [file si.pdf]

# Supporting Information: Transferability of Atom-Based Neural Networks

Frederik Ø. Kjeldal and Janus J. Eriksen*

*DTU Chemistry, Technical University of Denmark*

*Kemitorvet Bldg. 206, 2800 Kgs. Lyngby, Denmark*

E-mail: janus@dtu.dk

# 1 Model Training

Two training configurations for models based either exclusively on total energies or a combination of these and corresponding atomic energies are supplied in the accompanying YAML files, `example_total.yaml` and `example_atom.yaml`. Please note that `optimizer_amsgrad` was turned on for the standard total energy model, as this may improve out-of-distribution transferability. For the models trained also on atomic energies from electronic-structure decompositions, both of the two arguments, `per_species_rescale_scales_trainable` and `per_species_rescale_shifts_trainable`, were set to true.

# 2 Additional Results

Table S1: Mean absolute errors upon moving away from the carbonyl functional group.

| Atom | Total Energy | IBO/IAO | EDA |
|---|---|---|---|
| C=**O** | 21.39 ± 2.00 | 47.56 ± 8.30 | 3.37 ± 3.27 |
| **C**=O | 6.96 ± 2.94 | 112.62 ± 6.46 | 6.23 ± 4.10 |
| 1 Bond | 6.34 ± 3.35 | 7.29 ± 2.90 | 5.62 ± 4.05 |
| 2 Bonds | 7.29 ± 3.63 | 1.70 ± 1.18 | 2.92 ± 2.18 |
| 3 Bonds | 6.42 ± 3.51 | 1.09 ± 0.96 | 1.37 ± 1.32 |

Table S2: Mean absolute errors upon moving away from the secondary amine group.

| Atom | Total energy | IBO/IAO | EDA |
|---|---|---|---|
| **N** | 16.72 ± 4.43 | 8.48 ± 12.93 | 6.61 ± 5.51 |
| 1 Bond | 5.99 ± 2.85 | 11.57 ± 8.00 | 4.33 ± 4.82 |
| 2 Bonds | 2.83 ± 1.94 | 1.03 ± 2.10 | 2.40 ± 3.31 |
| 3 Bonds | 2.87 ± 2.07 | 0.74 ± 0.77 | 1.04 ± 1.43 |
| 4 Bonds | 2.62 ± 1.55 | 0.36 ± 0.41 | 0.55 ± 0.79 |

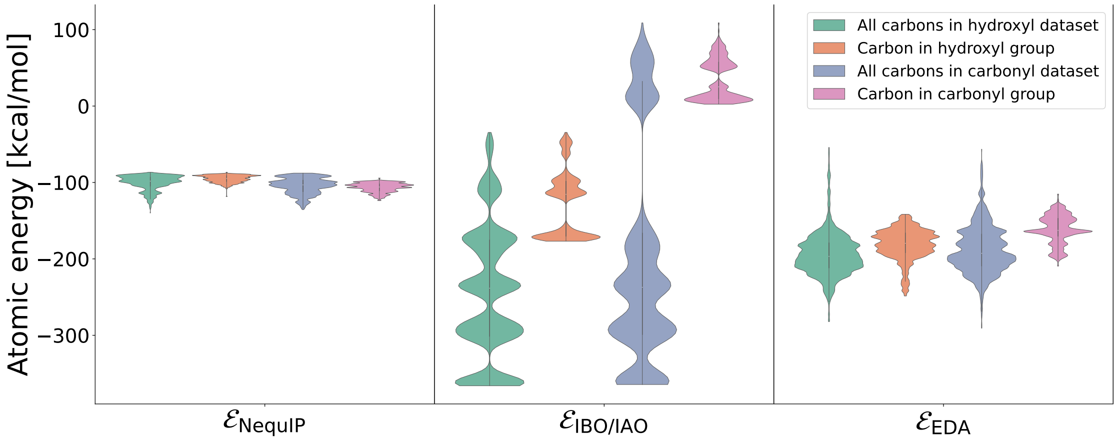


Figure S1: Detailed look at the carbon distributions in Fig. 3 of the main study.

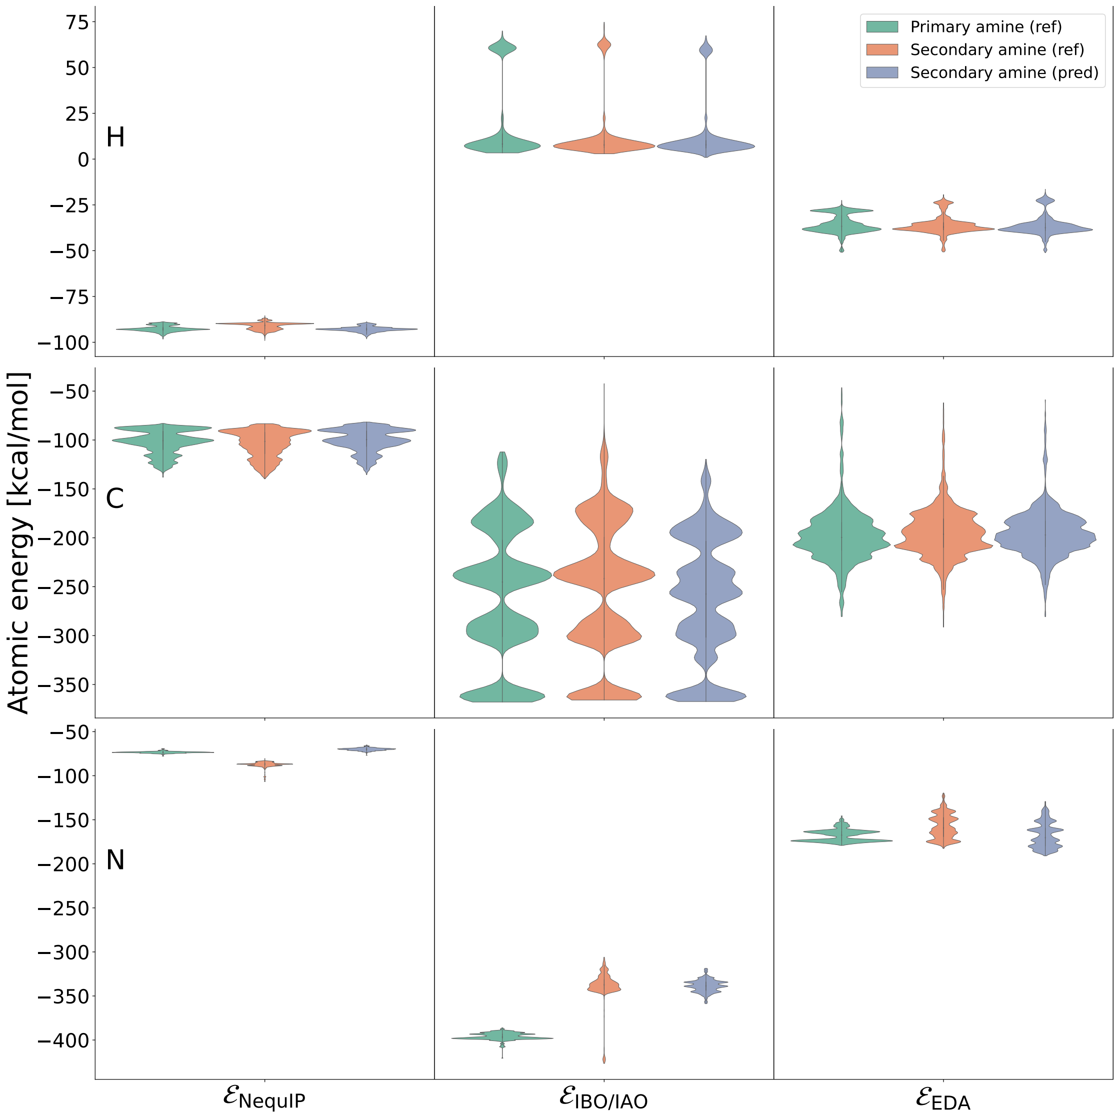


Figure S2: Same as Fig. 3, but for the datasets of primary and secondary amines.

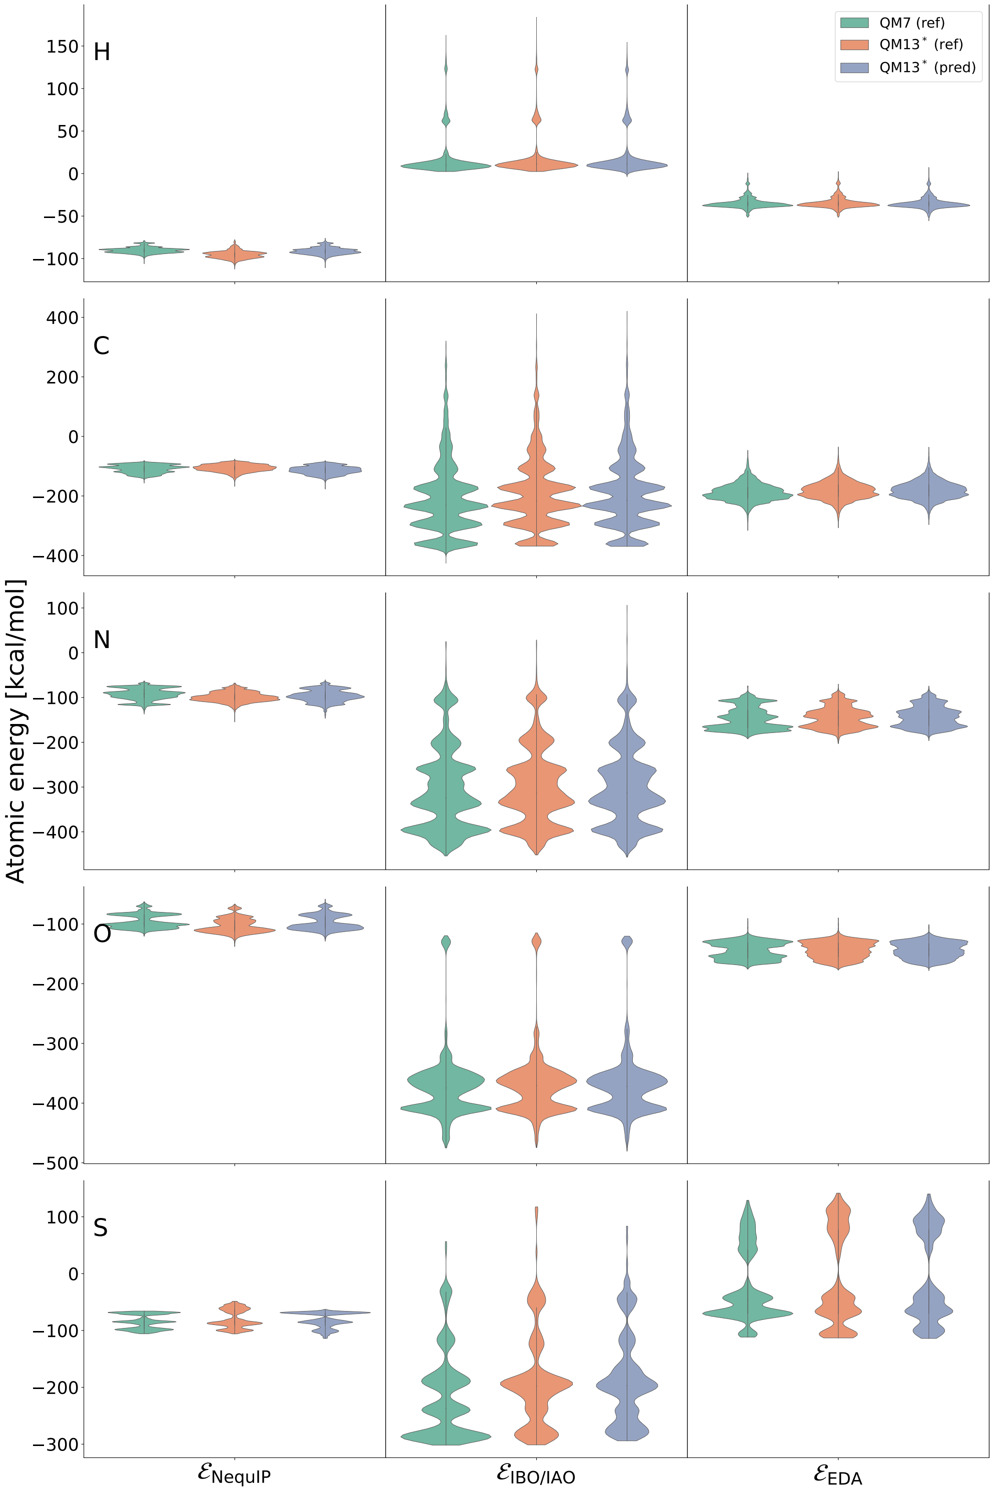


Figure S3: Same as Fig. 3, but for the QM7 and QM13* datasets.

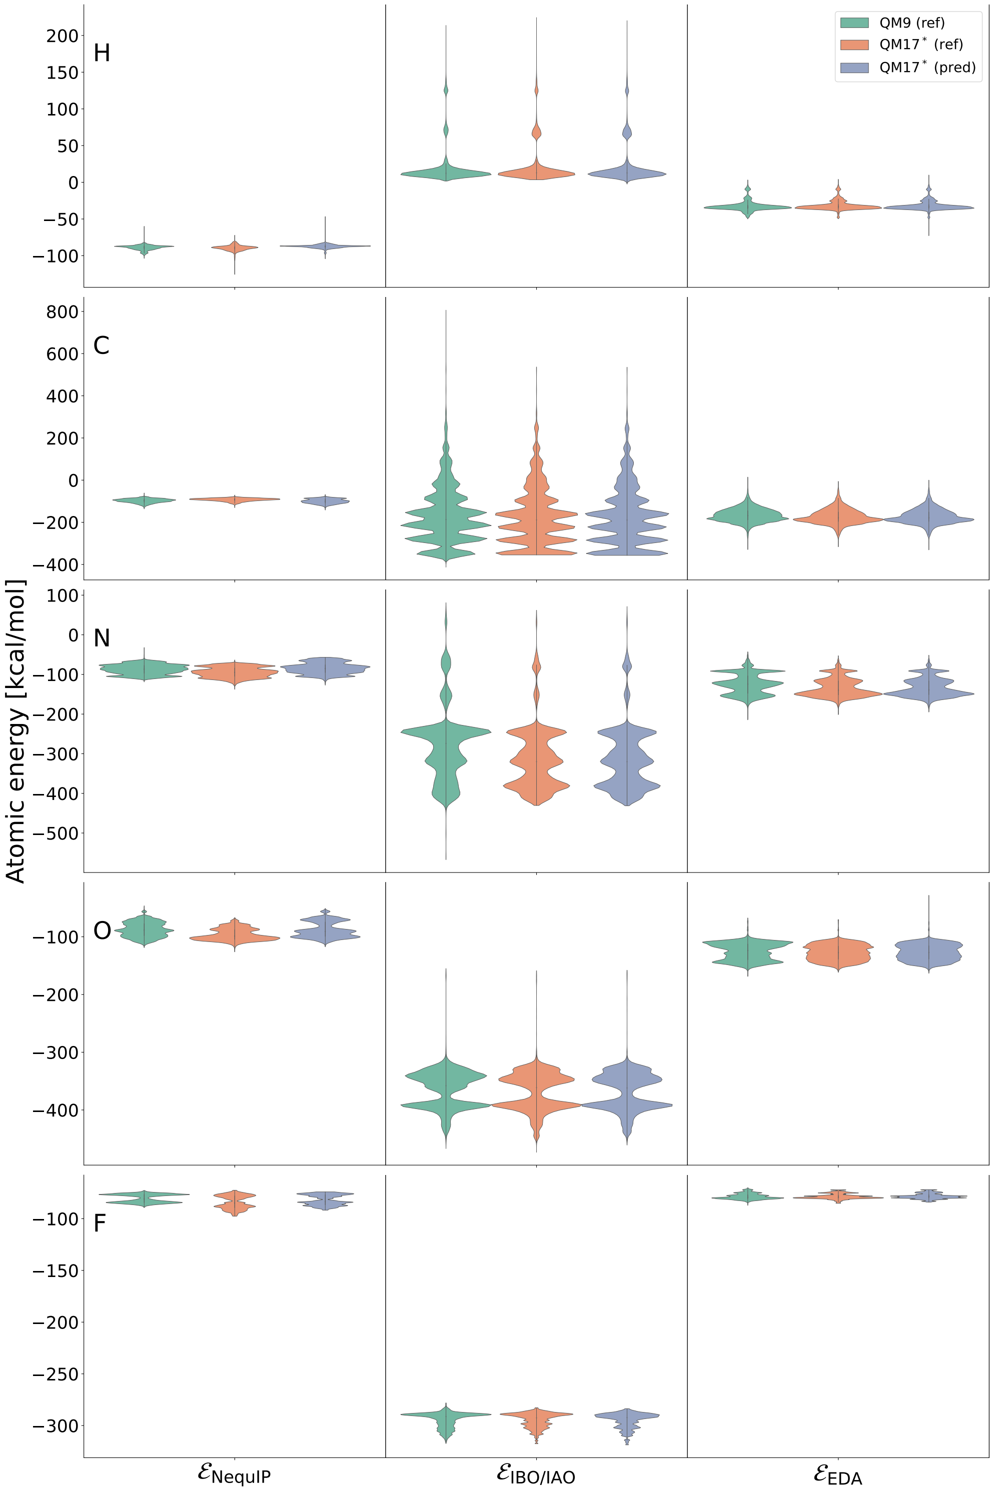


Figure S4: Same as Fig. 3, but for the QM9 and QM17* datasets.

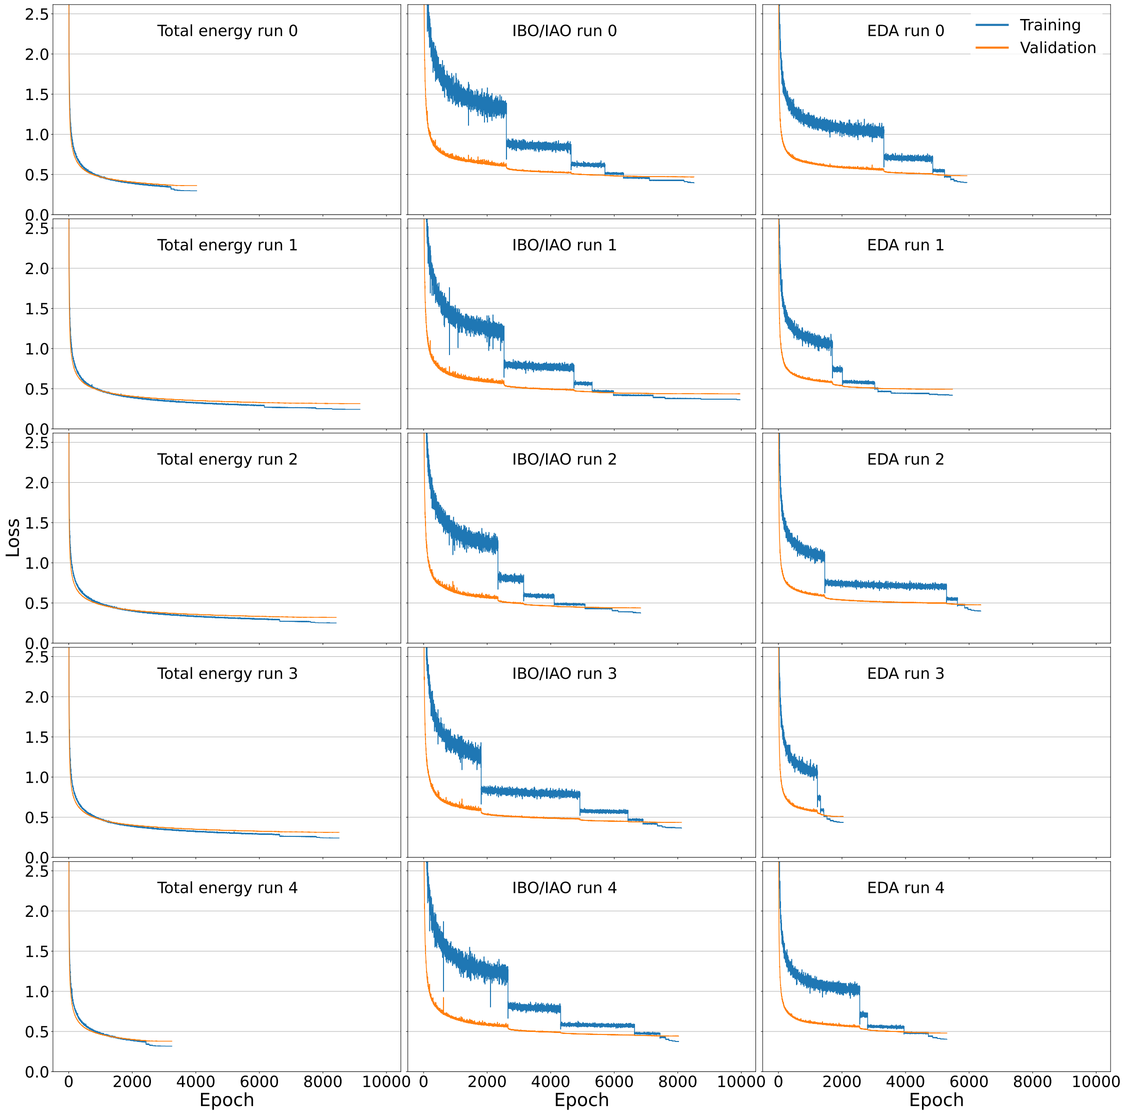


Figure S5: The training curves of the $l_{max} = 0$ models trained on the QM9 dataset.

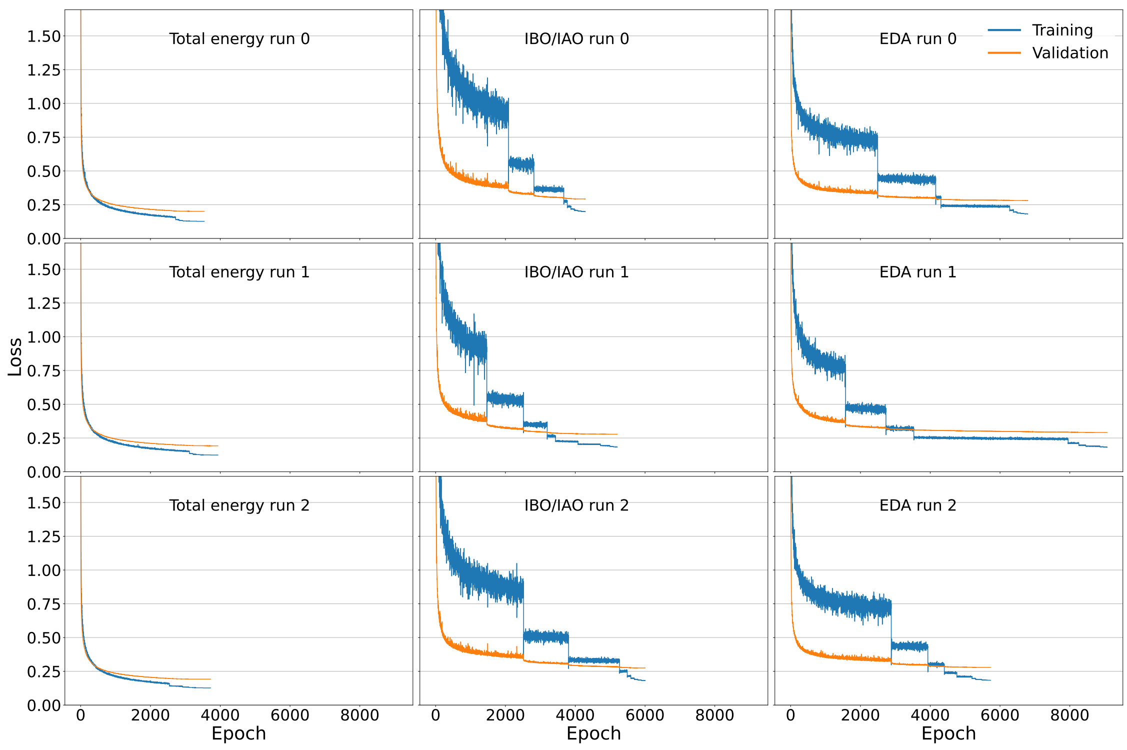


Figure S6: The training curves of the $l_{max} = 1$ models trained on the QM9 dataset.

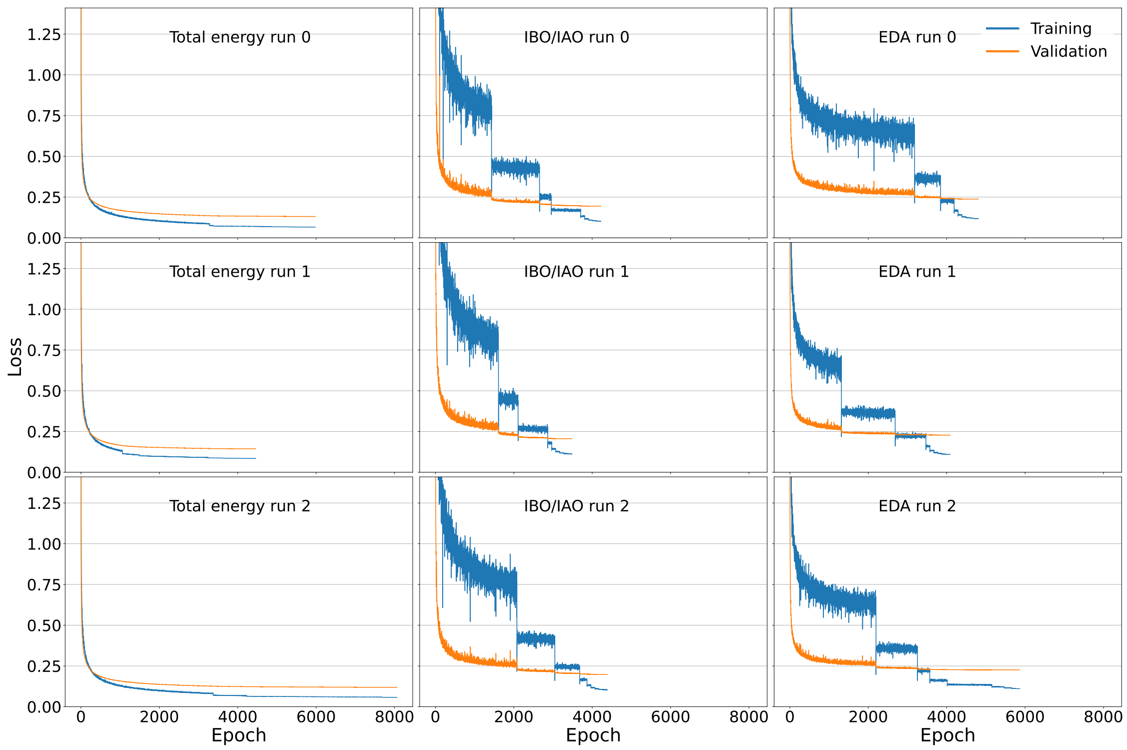


Figure S7: The training curves of the $l_{max} = 2$ models trained on the QM9 dataset.

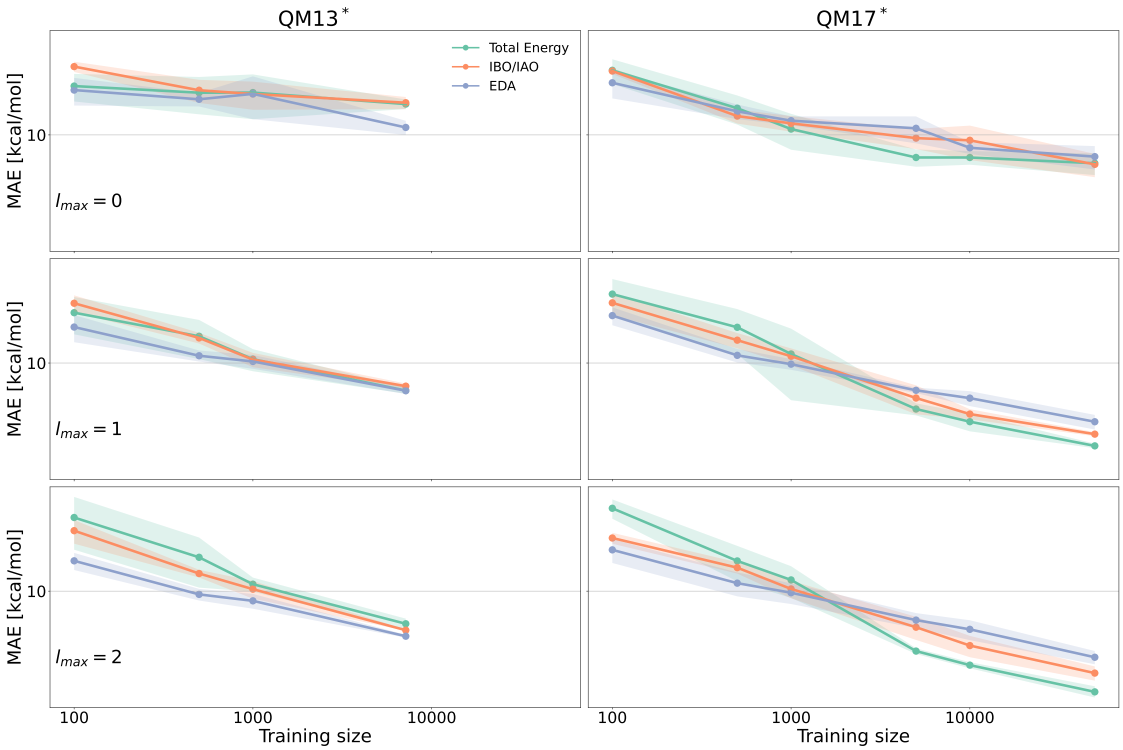


Figure S8: MAEs for QM13*/17* when training on increasing shares of QM7/9.

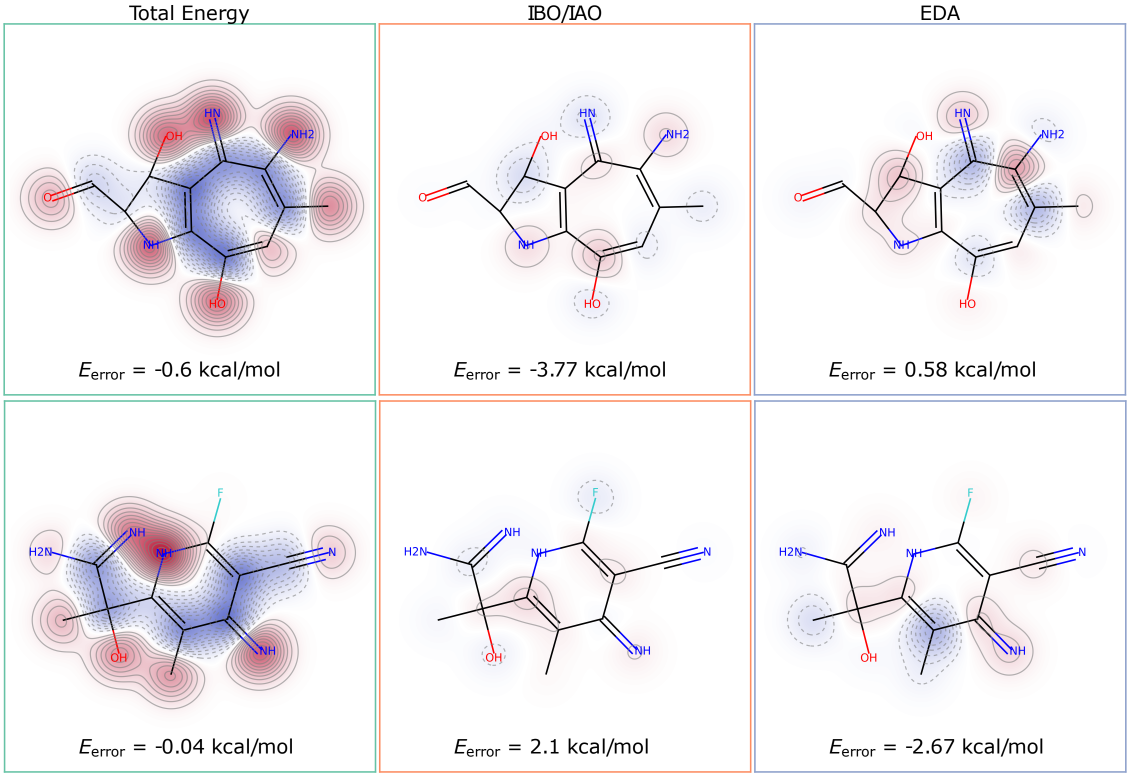


Figure S9: Same as Fig. 5 but for two other entries of the QM17* dataset.

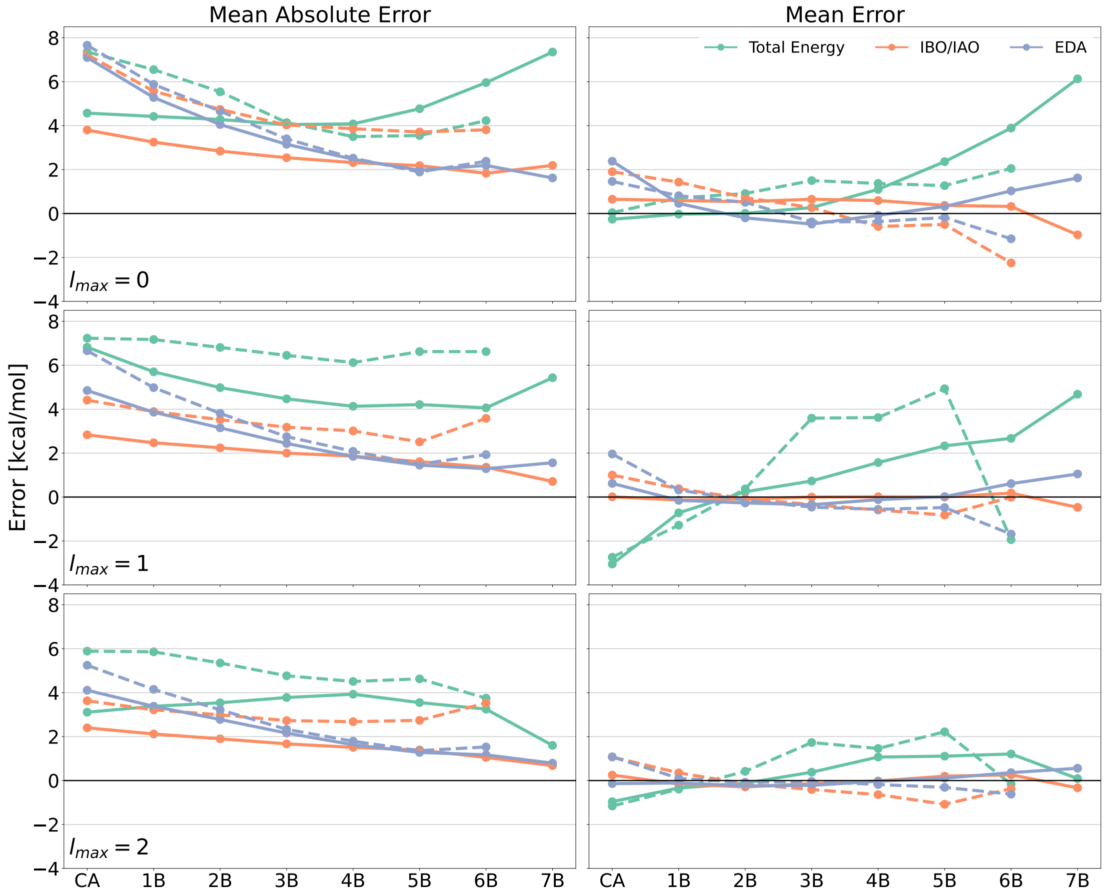


Figure S10: Same as Fig. 6 but with a reduced QM9 training size of 10,000 molecules.
